# Supplementary material for: Asymmetry in Polymer-Solvent Interactions Yields Complex Thermoresponsive Behavior
Source: arXiv:2312.00940 source file (2024-03-01)
Supplement: Supplementary file 2 [file packages_supp.tex]

\setlength{\oddsidemargin}{0in}  %left margin position, reference is one inch
\setlength{\textwidth}{6.5in}    %width of text=8.5-1in-1in for margin
\setlength{\topmargin}{-0.5in}    %reference is at 1.5in, -.5in gives a start of about 1in from top
\setlength{\textheight}{9in}     %length of text=11in-1in-1in (top and bot. marg.) 

\usepackage{amsmath,amssymb, mathtools}
\usepackage{titlesec}
\titleformat{\section}
  {\normalfont\fontsize{14}{15}\bfseries}{\thesection}{1em}{}
\titleformat*{\subsection}{\small\bfseries}
\titleformat*{\subsubsection}{\small\bfseries}

\usepackage{graphicx}% Include figure files
\usepackage{dcolumn}% Align table columns on decimal point
\usepackage{bm}% bold math
\usepackage{upgreek}
\usepackage[numbers,super,comma,sort&compress]{natbib}
\usepackage{lipsum}  
\usepackage{tabularx}
\usepackage{booktabs}
\usepackage{enumitem}
\usepackage{setspace}
\usepackage{array}
\usepackage[makeroom]{cancel}
\usepackage{empheq}
\newcommand\widecolourbox[1]{{\setlength\fboxrule{1pt}\setlength\fboxsep{8pt}\fcolorbox{black}{white}{\enspace#1\enspace }}}


% USER COMMANDS
% \newcommand{\mySection}[1]{\section*{\sffamily\Large\thesection\ #1}\vspace{-0.5em}\hrule\vspace{0.5em}}
% \newcommand{\mySection}[1]{\section*{\fontfamily{phv}\selectfont #1}}
\newcommand{\smallerSection}[1]{\titleformat{\section}{\large\bfseries\filcenter}{\thesection}{1em}{\MakeUppercase{#1}}}
\newcommand{\mySection}[1]{\section*{\sffamily \large {#1}}}
\newcommand{\mySubSection}[1]{\section*{\sffamily \normalsize {#1}}}

\DeclareRobustCommand*{\citen }[1]{%
  \begingroup
    \romannumeral-`\x % remove space at the beginning of \setcitestyle
    \setcitestyle{numbers} %
    \cite{#1} %
  \endgroup   
}
\usepackage{xcolor}
% \usepackage[dvipsnames]{xcolor}
% \newcommand{\sd}[1]{\textcolor{black}{#1}}
% \newcommand{\maw}[1]{\textcolor{black}{#1}}

\usepackage[parfill]{parskip}    % Activate to begin paragraphs with an empty line rather than an indent

\usepackage{wasysym}
\usepackage[font=footnotesize]{caption}
\usepackage{float}
\usepackage{capt-of}
\usepackage{helvet}
\usepackage{enumitem}
\usepackage{relsize}
\usepackage{makecell}

\makeatletter
\newcommand*{\addFileDependency}[1]{
  \typeout{(#1)}
  \@addtofilelist{#1}
  \IfFileExists{#1}{}{\typeout{No file #1.}}
}
\makeatother
\newcommand*{\myexternaldocument}[1]{
    \externaldocument{#1}
    \addFileDependency{#1.tex}
    \addFileDependency{#1.aux}
}
% put all the external documents here!
% \myexternaldocument{main}
